# Supplementary material for: The Role of Large Language Models in the Recognition of Territorial Sovereignty: An Analysis of the Construction of Legitimacy
Source: arXiv:2304.06030 source file (2023-04-18)
Supplement: Supplementary file 2 [file appendix.tex]

\section*{Appendix}\label{sec:appendix}
